# Supplementary material for: FLASH-FHE: A Heterogeneous Architecture for Fully Homomorphic Encryption Acceleration
Source: arXiv:2501.18371 source file (2025-01-30)
Supplement: Supplementary file 1 [file 4x4_transpose_end.tex]

\begin{table}[H]
\centering
\begin{tabular}{c|c|c|c|c}
\toprule
	& Depth 0 & Depth 1 & Depth 2 & Depth 3\\
\hline
Port 0 & 0 & 1 & 2 & 3 \\
\hline
Port 1 & 4 & 5 & 6 & 7 \\
\hline
Port 2 & 8 & 9 & 10 & 11 \\
\hline
Port 3 & 12 & 13 & 14 & 15 \\
\bottomrule
\end{tabular}
\caption{Target state of a $4\times 4$ transpose example.}
\label{tab:transpose_end}
\end{table}
