# Supplementary material for: FLASH-FHE: A Heterogeneous Architecture for Fully Homomorphic Encryption Acceleration
Source: arXiv:2501.18371 source file (2025-01-30)
Supplement: Supplementary file 2 [file 4x4_transpose_init.tex]

\begin{table}[H]
\centering
\begin{tabular}{c|c|c|c|c}
\toprule
	& Depth 0 & Depth 1 & Depth 2 & Depth 3\\
\hline
Port 0 & 0 & 4 & 8 & 12 \\
\hline
Port 1 & 1 & 5 & 9 & 13 \\
\hline
Port 2 & 2 & 6 & 10 & 14 \\
\hline
Port 3 & 3 & 7 & 11 & 15 \\
\bottomrule
\end{tabular}
\caption{Initial state of a $4\times 4$ transpose example.}
\label{tab:transpose_init}
\end{table}
