# Supplementary material for: FLASH-FHE: A Heterogeneous Architecture for Fully Homomorphic Encryption Acceleration
Source: arXiv:2501.18371 source file (2025-01-30)
Supplement: Supplementary file 3 [file 4x4_transpose_workflow.tex]

\newcommand{\CC}[1]{\cellcolor{blue!#1}}
\begin{table*}[t]
\centering
\begin{tabular}{c|c|c|c|c|c|c|c|c|c}
\toprule
	& Cycle 0 & Cycle 1 & Cycle 2 & Cycle 3 & Cycle 4 & Cycle 5 & Cycle 6 & Cycle 7 & Cycle 8 \\
\hline
Port 0 & \CC{20}0 & \CC{20}4 & \CC{20}8 & \CC{20}12 & \CC{20} & \CC{20} & \CC{20} & \CC{20} & \CC{20} \\
Port 1 & \CC{20} & \CC{20} 1 & \CC{20} 5 & \CC{20} 9 & \CC{20} 13 & \CC{20} & \CC{20} & \CC{20} & \CC{20} \\
Port 2 & \CC{20} & \CC{20} & \CC{20} 2 & \CC{20} 6 & \CC{20} 10 & \CC{20} 14 & \CC{20} & \CC{20} & \CC{20} \\
Port 3 & \CC{20} & \CC{20} & \CC{20} & \CC{20} 3 & \CC{20} 7 & \CC{20} 11 & \CC{20} 15 & \CC{20} & \CC{20} \\
\hline
MUX 0 & 0 & 1 & 8 & 9 & & & & &  \\
MUX 1 & & 4 & 5 & 12 & 13 & & & & \\
MUX 2 & & & 2 & 3 & 10 & 11 & & & \\
MUX 3 & & & & 6 & 7 & 14 & 15 & &  \\
\hline
Reg 0 & & 0 & 1 & 8 & 9 & & & &  \\
Reg 1 & & & 4 & 5 & 12 & 13 & & & \\
Reg 2 & & & & 2 & 3 & 10 & 11 & & \\
Reg 3 & & & & & 6 & 7 & 14 & 15 & \\
\hline
MUX 4 & & 0 & 1 & 2 & 3 & & & & \\
MUX 5 & & & 4 & 5 & 6 & 7 & & & \\
MUX 6 & & & & 8 & 9 & 10 & 11 & & \\
MUX 7 & & & & & 12 & 13 & 14 & 15 & \\
\hline
Reg 4 & & & 0 & 1 & 2 & 3 & & &  \\
Reg 5 & & & & 4 & 5 & 6 & 7 & &  \\
Reg 6 & & & & & 8 & 9 & 10 & 11 &  \\
Reg 7 & & & & & & 12 & 13 & 14 & 15  \\
\bottomrule
\end{tabular}
\caption{Detailed workflow of the $4\times 4$ transpose example. The blue part shows the data distribution after delay module.}
\label{tab:transpose_example}
\end{table*}
